# Supplementary material for: On Designing Consistent Covariance Recovery from a Deep Learning Visual Odometry Engine
Source: arXiv:2403.13170 source file (2024-03-19)
Supplement: Supplementary file 1 [file appendix.tex]

\section{Derivation of Jacobians}
